# Supplementary material for: Behavioral Learning of Dish Rinsing and Scrubbing based on Interruptive Direct Teaching Considering Assistance Rate
Source: arXiv:2408.09360 source file (2024-12-21)
Supplement: Supplementary file 1 [file appendix.tex]

\section*{Appendix}

Appendix
